# Supplementary material for: Superconducting Graphene: the conspiracy of doping and strain
Source: arXiv:1308.2566 source file (2013-08-12)
Supplement: Supplementary file 1 [file Superconducting-Graphene-supplementary-information.pdf]

**Supplementary information**

# Superconducting Graphene: the conspiracy of doping and strain


Chen Si,[1,2†] Zheng Liu,[2†] Wenhui Duan,[1] & Feng Liu[2]*

[1]Department of Physics and State Key Laboratory of Low-Dimensional Quantum Physics, Tsinghua University, Beijing 100084, People's Republic of China

[2]Department of Materials Science and Engineering, University of Utah, Salt Lake City, UT 84112, USA

[†]These authors contributed equally to this work.

*Email: fliu@eng.utah.edu


## 1. Computational Method

Our calculations are performed using first-principles density functional theory method within local density approximation as implemented in the QUANTUM-ESPRESSO code [S1]. Graphene layers are separated by 15 Å of vacuum to eliminate the interlayer interaction. The charge doping is simulated by adding or removing electrons to the graphene with a compensating uniform charge background of opposite sign. Norm-conserving pseudopotentials with a plane-wave cutoff energy of 80 Ry are used to describe the electron-ion interaction. The electronic integration is approximated by a summation over a 90×90×1 k-mesh with a Methfessel-Paxton smearing [S2] of 0.02 Ry for the self-consistent cycles. The Dynamic matrixes are calculated on an 18×18×1 q-mesh. A much finer k-mesh (180×180×1) is used for obtaining the electron-phonon coupling parameter $\lambda$.

## 1. $\omega_{\log}$ as a function of strain

To calculate $T_c$, we have first calculated $\omega_{\log}$ as a function of doping and strain $\varepsilon$, which is found almost independent of doping but a strong function of strain as shown in Fig. S1.

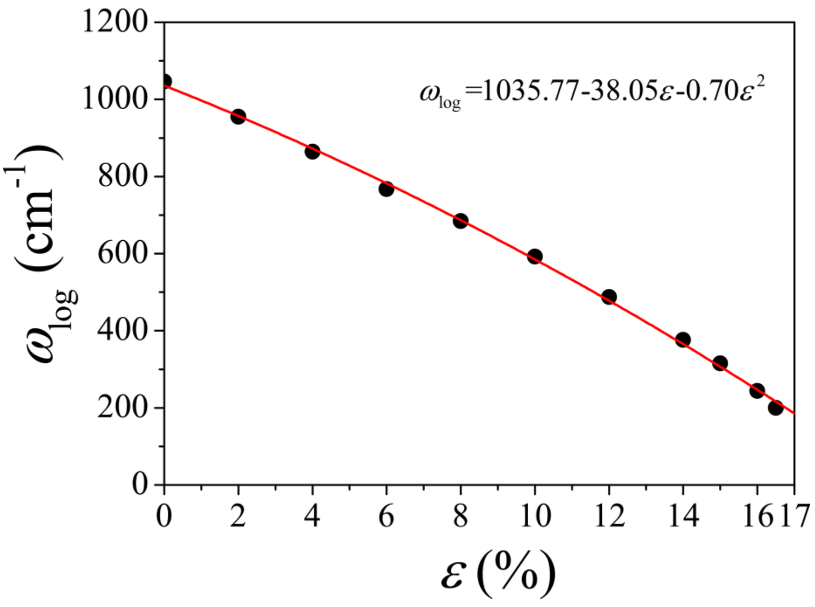


**Fig. S1** **$\omega_{log}$ versus ε for the $4.65\times10^{14}$ cm$^{-2}$ hole-doped graphene.** The calculated data of $\omega_{log}$-$\varepsilon$ (black dots) can be nicely fitted to the second order of strain (red line).

## 2. Evaluation of $\mu^*$ in graphene

Similar to λ, the dimensionless coefficient of screened Coulomb potential is defined by the average strength of Coulomb potential on the Fermi surface, $\mu = N_F V_{ee}$. When the characteristic electron energy ($\omega_e$) is much larger than the phonon energy ($\omega_D$), the retardation effect should be taken into account, which scales down the Coulomb potential, giving the retarded form of the Coulomb pseudopotential $\mu^*$ used in Eq. (9) as

$$\mu^* = \frac{\mu}{1+\mu\ln(\omega_e/\omega_D)} \tag{s1}$$

We can analytically evaluate $\mu$ and $\mu^*$, starting from the single-particle effective Hamiltonian around $K$ and $K'$ points for graphene,

$$H_o = \sum_{k_0=K,K'}\sum_p v_0 |p| c^+_{k_0+p} c_{k_0+p} \tag{s2}$$

The eigenstates can be obtained as

$$\psi_p(r) = \frac{1}{\sqrt{2}}\begin{pmatrix} -ie^{-i\frac{\theta_p}{2}} \\ e^{i\frac{\theta_p}{2}} \end{pmatrix} \exp[i(k_0+p)\cdot r] \tag{s3}$$

The bare Coloumb potential in the momentum space is then

$$V_{ee}(q) = \iint dr dr' \frac{\psi^*_{p+q}(r)\psi_p(r)\psi^*_{p'-q}\psi_{p'}(r')}{|r-r'|} = (1-\frac{q^2}{4p_F^2})\frac{2\pi}{q} \tag{s4}$$

To perform the average of the screened Coulomb potential on the Fermi surface, we neglect

the inter-valley interaction because it relates to large momentum $q$, and hence much smaller than the intra-valley component. We adopt the dielectric function of graphene as obtained by Hwang and Das Sarama [S3]:

$$\epsilon(q) = \kappa + \frac{4\pi}{q} N(E_F) \tag{s5}$$

in which $\kappa$ is the dielectric constant, which in experiment depends on the substrate of graphene

$$\mu = \langle V_{ee}^{sc} \rangle_{FS} = \oint_{FS} dp_F \oint_{FS} dp_F' \frac{V_{ee}(p_F - p_F')}{\epsilon(p_F - p_F')} = \frac{1}{\pi}\int_0^{\pi} d\tilde{\theta} \frac{\cos^2\tilde{\theta}}{\kappa v_0 \sin\tilde{\theta} + 2} \tag{s6}$$

We note than $\mu$ is a strong function of dielectric constant ($\kappa$) and Fermi velocity $v_0$, but a weak function of Fermi level of strain, especially in the regime of linear energy dispersion. We plot the $\mu \sim \kappa v_0$ relationship in Fig. S2. For the realistic case, we use $v_0$ = c/300 and $\kappa$ = 2.5 which corresponds to a conventional $SiO_2$ substrate. These parameters give $\mu$ = 0.21. If we neglect the small change of Fermi velocity by doping and strain, then we can approximately treat $\mu$ as a constant. When the Fermi velocity by doping and strain, then we can approximately treat $\mu$ as a constant. When the Fermi energy is larger than the Debye energy ($\omega_D$ ~ 0.2 eV), we will include the retardation effect (Eq. s1). This would give an explicit formula for $\mu^*$ as

$$\mu^*(E_F) = \begin{cases} 0.21 & E_F < 0.2 \\ \dfrac{0.21}{1 + 0.21\ln(5E_F)} & E_F \geq 0.2 \text{ e} \end{cases} \tag{s7}$$

We plot the $\mu^* \sim \kappa v_0$ in Fig. S2 along with $\mu$. The $\mu^*$ in graphene falls typically in the range of ~0.10-0.15, consistent with the reported values in other carbon-related materials and most sp-electron metals.

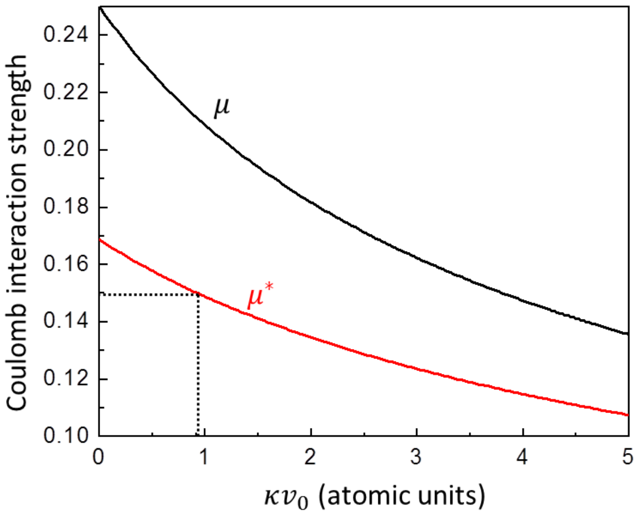


**Fig. S2** **$\mu$ and $\mu^*$ of graphene as a function of $\kappa v_0$.** $\mu^*$ is evaluated by choosing $E_F$ = 1 eV.

**Table S1. The calculated $\lambda$, $\omega_{\log}$ and $T_c$ of the 4.65 $\times 10^{14}$ cm$^{-2}$ electron/hole doped graphene under different biaxial tensile strain.**

| Strain ($\varepsilon$) (%) | $\lambda$ | | $\omega_{\log}$ (cm$^{-1}$) | | $T_c$ (K) ($\mu$*=0.1) | | $T_c$ (K) ($\mu$*=0.15) | |
|---|---|---|---|---|---|---|---|---|
| | *p-type* | *n-type* | *p-type* | *n-type* | *p-type* | *n-type* | *p-type* | *n-type* |
| 0.0 | 0.14 | 0.09 | 1054.0 | 1048.5 | 0 | 0 | 0 | 0 |
| 12 | 0.41 | 0.26 | 491.0 | 579.7 | 3.4 | 0.1 | 0.8 | 0 |
| 13 | 0.49 | 0.32 | 441.0 | 506.2 | 7.2 | 0.6 | 2.8 | 0.03 |
| 15 | 0.76 | 0.54 | 317.2 | 344.4 | 19.4 | 8.0 | 13.0 | 3.7 |
| 16 | 1.11 | 0.85 | 245.7 | 245.4 | 28.4 | 18.4 | 22.6 | 13.1 |
| 16.5 | 1.45 | 1.20 | 200.9 | 185.4 | 31.6 | 23.8 | 26.8 | 19.3 |

**Reference**


S1. P. Giannozzi, S. Baroni, N. Bonini, M. Calandra, R. Car, C. Cavazzoni, D. Ceresoli, G. L. Chiarotti, M. Cococcioni and I. Dabo, *J. Phys.: Condens. Matter*, **21**, 395502 (2009).

S2. M. Methfessel and A. Paxton, *Phys. Rev. B* **40**, 3616 (1989).

S3. Hwang, E. H. & Das Sarma, S. Dielectric function, screening, and plasmons in two-dimensional graphene. *Phys. Rev. B* **75**, 205418 (2007).
